# Supplementary material for: X-Pose: Detecting Any Keypoints
Source: arXiv:2310.08530 source file (2024-07-17)
Supplement: Supplementary file 1 [file supp.tex]

\section{Details in the UniKPT Dataset}
\label{sec:supp_data}
As shown in Fig.~\ref{fig:dataset}, we demonstrate that each dataset only focuses on a single super-category (e.g., ``human only'' and ``animal only''), making it challenging to achieve keypoint generalization when using them individually. Additionally, these datasets have significant differences in the quality, quantity, and appearance styles of keypoint annotations. Therefore, we are motivated to unify all the datasets into one called {UniKPT}, following the below guidelines:

\begin{figure*}[h]	
\centering
 	{
 			\centering         
 			\includegraphics[width=1.0\linewidth]{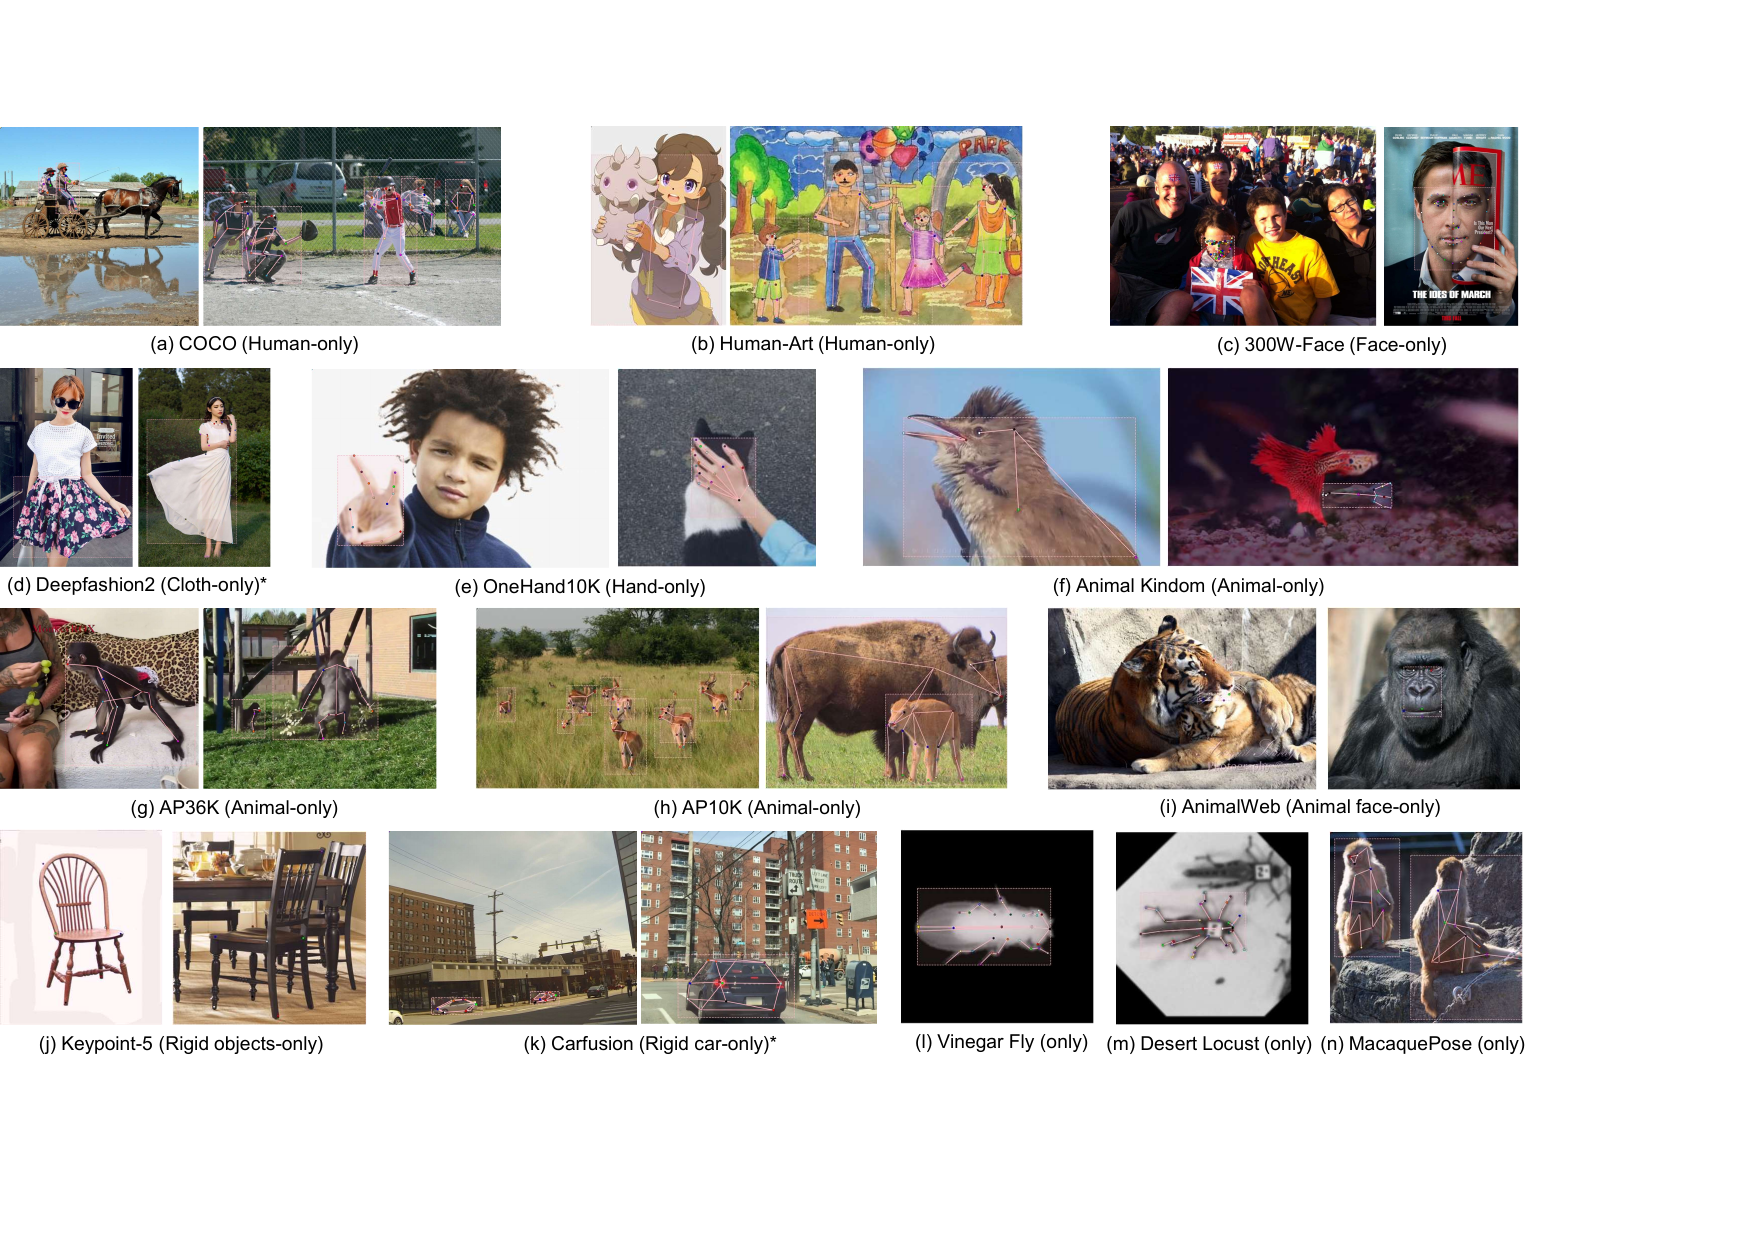}   
 	} 
\vspace{-0.5cm}
\caption{Visualization the unified dataset ({UniKPT}) for each original dataset. * means the two datasets are included in MP-100~\cite{xu2022pose}.
}
\label{fig:dataset} 
% \vspace{-0.3cm}
\end{figure*}

\noindent \textbf{Annotating Detailed Keypoint Descriptions.} 
The majority of keypoints in existing datasets lack detailed annotations to distinguish between different keypoints. For example, in the DeepFashion2 dataset~\cite{ge2019deepfashion2}, keypoints are identified solely by numerical labels (e.g., 1, 2, 3, 4) for clothing items. To benefit the fine-grained text-to-keypoint alignments, we annotate each keypoint with comprehensive textual descriptions, incorporating rich directional information such as `upper', `lower', `left', and `right', and assigning each keypoint a unique name to add the fine-grained semantic meaning and prevent any conflicts.

\noindent \textbf{Unifying Keypoint's Textual Description.} Given that descriptions for the same keypoint may vary across different datasets, we standardize the names of overlapping keypoints. To this end, we could align fine-grained keypoint features that share similar local visual patterns, such as \textit{``the left eye of humans''} and \textit{``the left eye of cats''}, by using a unified textual description.

\noindent \textbf{Unifying Orientation Criterion.} We observe discrepancies in existing datasets regarding the definition of left and right orientations. Thus, we standardize left and right orientation definitions based on the object's left and right within the image, which can promote the alignment of directional information between the text and keypoints.

\noindent \textbf{Balancing Data Volume and Object Categories.}
Among the $13$ datasets, we have used the entire dataset for most of them because they encompass a diverse range of multi-object scenarios (e.g., COCO~\cite{lin2014microsoft}), varied photo styles (e.g., Human-Art~\cite{ju2023human}), or a large number of species categories (e.g., AnimalKindom~\cite{ng2022animal}). However, for some datasets such as Onehand10K~\cite{wang2018mask} for the human hand, MacaquePose\cite{labuguen2021macaquepose} for macaque animals, and Keypoint-5~\cite{wu2016single} for furniture, each only containing single-object scenes featuring limited categories, we randomly sample $2,000$ images from each for training.

\section{More Experiments}

\subsection{Comparison with Open-set Object Detector-Grounding-DINO}
\noindent \textbf{Implementation Details.} Directly using the keypoint-level textual prompt in Grounding-DINO~\cite{liu2023grounding} only outputs a set of keypoints without knowing which object these keypoints belong to. However, multi-object keypoint detection task needs to detect both the bounding boxes of individual objects and their corresponding keypoints. Thus, we conduct two steps for evaluation: Firstly, we utilize the object-level textual prompt to detect all candidate object boxes. Then, we employ these object boxes to crop the images into individual single-object images. Secondly, we use the keypoint-level textual prompt to perform keypoint detection on these single-object images, wherein we select the top-1 score's box center as the keypoint position.

\noindent \textbf{Analysis.} We compare \ModelName with the state-of-the-art open-vocabulary object detector, Grounding-DINO, with a specific focus on object-level and keypoint-level detection in Tab.~\ref{tab:gd_complete}. \textbf{For object detection,} the original Grounding-DINO performs admirably on COCO since it has knowledge of the person categories. However, its performance sharply drops when the image style shifts to artificial scenes and when detecting the 54 different animal categories. After fine-tuning Grounding-DINO using the keypoint detection datasets, its detection performance on Human-Art and AP-10K has significantly improved. \ModelName has also achieved comparable detection performance to the fine-tuned Grounding-DINO model. \textbf{For keypoint detection}, while Grounding-DINO fails to localize fine-grained keypoint, \ModelName successfully addresses these challenges, achieving significant performance across all datasets.

\begin{table*}[t]
    \setlength\tabcolsep{6pt}
			\caption{Comparisons with the state-of-the-art open-set object detector, focusing on object-level and keypoint-level detection. $\ddag$ denotes the fine-tuning of GroundingDINO using the keypoint detection datasets. Notably, we limit the object-level comparison to $AP_{M}$ (medium objects) and $AP_{L}$ (large objects), as small objects do not have keypoints annotated. \textit{T} and \textit{V} denotes textual prompts and visual prompts used.}
   \vspace{-0.5cm}
	\begin{center}
\resizebox{\linewidth}{!}{
     % \begin{threeparttable}   
		\begin{tabular}{l|c|cc|ccc|c|c}
			\hline
                        \multirow{2}{*}{Methods} &  \multirow{2}{*}{Backbone}    &   \multicolumn{2}{c|}{object-level} & \multicolumn{3}{c|}{Keypoint-level} & \multirow{2}{*}{Training Datasets} & \multirow{2}{*}{Dataset Volume} \\
			  &  & ${\rm AP}_{M}$ & ${\rm AP}_{L}$ &${\rm AP}$ &  ${\rm AP}_{M}$ & ${\rm AP}_{L}$  &  & \\ \hline
                \multicolumn{9}{l}{\textit{\cellcolor{Gray!25} COCO \texttt{val} set}} \\
               GroundingDINO-\textit{T} & Swin-T & 70.8 & 82.0 &  3.1  & 2.8 & 3.2 & O365,GoldG,Cap4M & 1858K \\
                GroundingDINO-\textit{T} & Swin-B & 69.7 & 79.5 & 6.8 &  6.6 & 7.2  & COCO,O365,GoldG,Cap4M,OpenImage,ODinW-35,RefCOCO &  -\\ 
                GroundingDINO$\ddag$-\textit{T} & Swin-T & \textbf{71.2} & \textbf{83.4} & 1.8  & 1.7 & 1.9 & COCO,Human-Art,AP-10K,APT-36K & 1858K  +  155K\\
                              \ModelName-\textit{T} & Swin-T & 71.1 & 80.2 & \textbf{74.2} & \textbf{68.8}  & \textbf{82.1} & COCO,Human-Art,AP-10K,APT-36K & 155K  \\
                \ModelName-\textit{V} & Swin-T & 71.1 & 80.3 & 74.1 & \textbf{68.8} & 81.8  & COCO,Human-Art,AP-10K,APT-36K & 155K  \\
                \multicolumn{9}{l}{\textit{\cellcolor{Gray!25} Human-Art \texttt{val} set}} \\
               GroundingDINO-\textit{T} & Swin-T &11.5 & 27.0  & 2.1 & 1.7 & 2.3
            & O365,GoldG,Cap4M & 1858K \\
               GroundingDINO-\textit{T} & Swin-B &  13.3&27.9  & 4.4  & 3.7 & 4.5  &COCO,O365,GoldG,Cap4M,OpenImage,ODinW-35,RefCOCO & - \\
                GroundingDINO$\ddag$-\textit{T} & Swin-T & 33.3 & \textbf{67.0} & 1.4 & 0.8 & 1.5  & COCO,Human-Art,AP-10K,APT-36K & 1858K  +  155K\\
                                \ModelName-\textit{T} & Swin-T & 33.7 &63.1   &  \textbf{72.2} & \textbf{39.5} & \textbf{76.7} & COCO,Human-Art,AP-10K,APT-36K & 155K  \\
                \ModelName-\textit{V} & Swin-T & \textbf{34.0} & 63.0  & 71.8 & 39.3& 76.4 & COCO,Human-Art,AP-10K,APT-36K & 155K  \\
                \multicolumn{9}{l}{\textit{\cellcolor{Gray!25} AP-10K \texttt{val} set}} \\
               GroundingDINO-\textit{T} & Swin-T  & 5.1 & 13.7  & 1.3 & 0.6 & 1.3 & O365,GoldG,Cap4M & 1858K \\
               GroundingDINO-\textit{T} & Swin-B & 29.1 & 44.1 &  7.8 & 5.4 & 8.2 & COCO,O365,GoldG,Cap4M,OpenImage,ODinW-35,RefCOCO & -\\
                GroundingDINO$\ddag$-\textit{T} & Swin-T & \textbf{56.5} & \textbf{79.7} & 0.7 &  0.4  & 1.0 & COCO,Human-Art,AP-10K,APT-36K & 1858K  +  155K\\
                \ModelName-\textit{T} & Swin-T &  54.5 & 78.8  & \textbf{73.2} & 45.6 & \textbf{74.3} & COCO,Human-Art,AP-10K,APT-36K & 155K  \\
            \ModelName-\textit{V} & Swin-T & 55.8 & 79.0 & 72.8 & \textbf{47.2} &74.0 & COCO,Human-Art,AP-10K,APT-36K & 155K  \\
             \hline
		\end{tabular}}

  \vspace{-0.2cm}
	\label{tab:gd_complete}
	\end{center}
\end{table*}

\begin{table*}[h]
	\begin{center}
 \caption{Comparisons with generalist models. TD and E2E are the top-down and end-to-end methods, respectively. }
\resizebox{0.7\linewidth}{!}{
  \begin{tabular}{l|ccc}
    \toprule
       \textbf{Method}& COCO \texttt{val} & HumanArt \texttt{val} & AP-10K \texttt{val}
\\ \hline
Unified-IO~\cite{lu2022unified} (TD)& 25.0 & 15.7 & 7.6  \\ 
Painter~\cite{wang2023images} (TD) & 70.2 & 12.4 &  15.3 \\ 
InstructDiffusion~\cite{geng2023instructdiffusion} (TD) &  71.2 &  51.4 & 15.9 \\ \hline
\ModelName-\textit{V} (E2E) &  \underline{76.6} &  \underline{75.5} & \underline{79.0} \\ 
\ModelName-\textit{T} (E2E) & \textbf{76.8} &  \textbf{75.9} & \textbf{79.2} \\ 
  \bottomrule
\end{tabular}
		}
  % \vspace{-0.3cm}
 \label{tab:generalist}	
 \end{center}
  \vspace{-0.7cm}
\end{table*}

\subsection{Comparison with Generalist Models}
We compare our \ModelName with several generalist models in terms of keypoint detection task as shown in Tab.~\ref{tab:generalist}.
Unlike these generalist models trained to handle multiple vision tasks, \ModelName targets an end-to-end keypoint generalist that could handle diverse multi-object and multi-class open-ended scenes. The results show that \ModelName outperforms all the generalist models across all evaluated keypoint datasets by a large margin.

\begin{figure*}[h]	
% \vspace{-0.2cm}
\centering
 	{
 			\centering         
 			\includegraphics[width=1.0\linewidth]{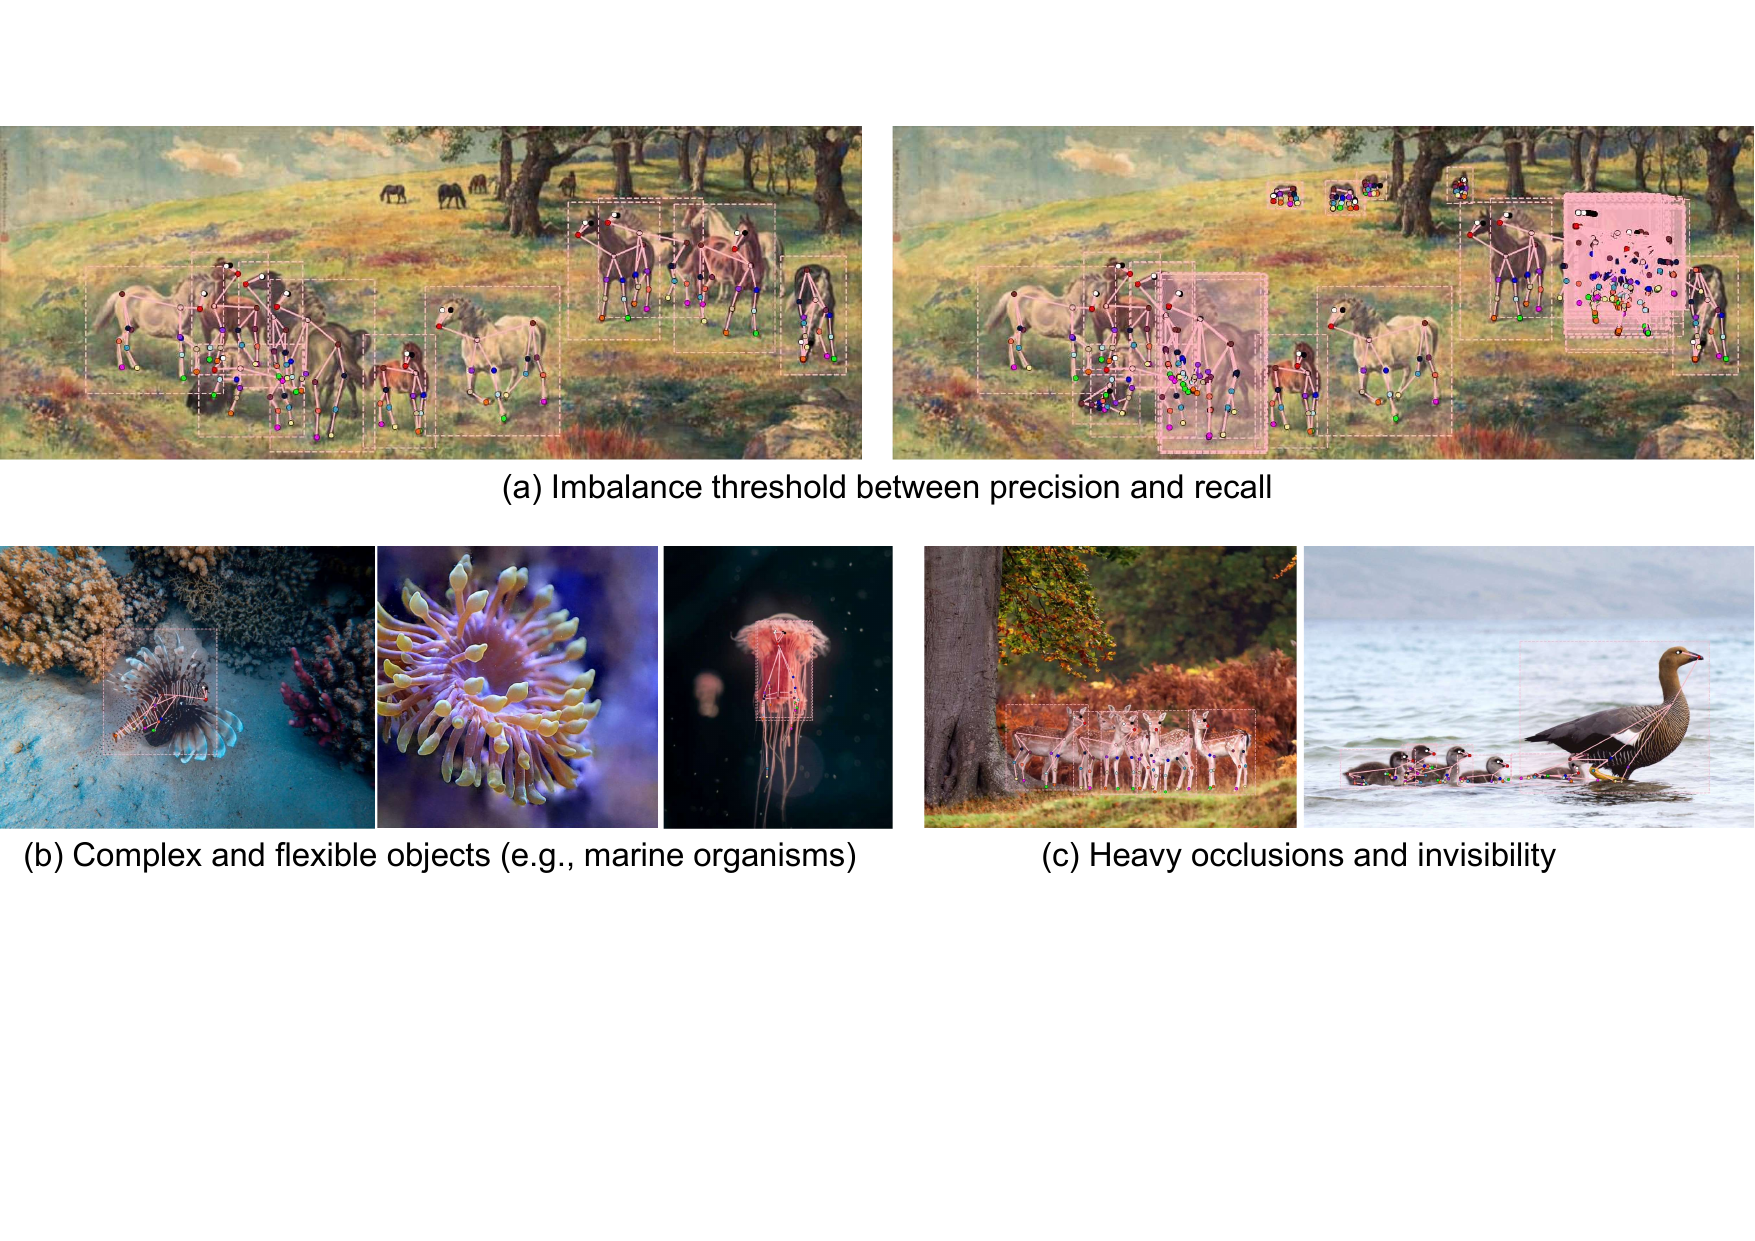}   
 	} 
\vspace{-0.5cm}
\caption{We show three types of failure cases in our method.
}
\label{fig:limitation} 
\vspace{-0.1cm}
\end{figure*}

\section{Discussion}
\label{sec:supp_conclusion}

\noindent \textbf{Failure Case Analysis.}
In Fig.~\ref{fig:limitation}, we show three kinds of failure cases in our method.
First, due to multi-object and multi-keypoint contrastive learning with textual prompts, the classification scores of instances and keypoints may be imbalanced across different categories. It will cause it to be hard to set a certain threshold for precise detection.
From the left figure of Fig.~\ref{fig:limitation}-(a), we set a higher threshold to demonstrate the outputs, and some objects are missing; we set a lower threshold, which will lead to some redundant detection. 
Second, despite the fact that we collected as many categories as possible, there are some keypoints of soft objects (\textit{e.g.}, marine organisms shown in Fig.~\ref{fig:limitation}-(b)) that are still difficult to define textually and visually, especially when only a single source image is inputted. These objects also tend to have similar local features in their visual appearance and global structural features that are not sufficiently distinct.
Third, Although our method shows superiority in multi-object detection scenarios, we find that recognition in places of extreme occlusion or heavily invisible keypoints, which may lose either local or global visual structure information, is still challenging (see Fig.~\ref{fig:limitation}-(c)).

\noindent \textbf{Limitation:}
In addition to the aforementioned failure case analysis, we believe the main issue currently lies in the data.
Although this work has aggregated $13$ keypoint datasets, there are still three limitations as follows:
\textbf{First}, compared with the amount of training data for CLIP~\cite{clip}, we still have $1,000$ times less data, leaving room for improvement in the performance and generalization of the model.
\textbf{Second}, some super-species with novel topologies that are not included (e.g., Kingdom Fungi and Kingdom Plantae) make the model hard to generalize to these cases.
\textbf{Lastly}, we did not consider fine-grained detection and segmentation datasets~\cite{shao2019objects365,he2022partimagenet} to strengthen the unified datasets. 
All the above issues will be left as future work.
